# Supplementary material for: A Markov Chain Model for Identifying Changes in Daily Activity Patterns of People Living with Dementia
Source: arXiv:2307.11126 source file (2023-07-20)
Supplement: Supplementary file 1 [file Supplementary_Information.tex]

In this section, we provide the supplementary evidence necessary to support our claims.

\subsection{Study Cohort Demographics}

Here we detail the distribution of diagnoses within the study cohort, as well as the variation in year of birth within the study cohort.

\begin{table}[H]
    \centering
    %\scriptsize
    \caption{Diagnoses for the study cohort}
     \begin{tabular}{c| c c c } 
         %\hline
         \toprule
         \textbf{Dementia Type} & \textbf{\%Male} & \textbf{\%Female} & \textbf{\%Total} \\ %[0.5ex] 
         %\hline
         \midrule
         \textbf{Alzheimer's Disease} & 34\% & 36\% & 70\% \\ 
         \textbf{Dementia with Lewy Bodies} & 3\% & 0\% & 3\%  \\
         \textbf{Frontotemporal Dementia} & 1.5\% & 1.5\% & 3\%  \\
         \textbf{Parkinson's Disease Dementia}  & 7\% & 0\% & 7\%  \\ 
         \textbf{Vascular Dementia} & 5\% & 0\% & 5\% \\
         \textbf{Other/Not specified} & 5\% & 7\% & 12\% \\
         %\hline
     \end{tabular}
     \label{tb:dementia_dignoses}
\end{table}

\begin{table}[H]
    \centering
    %\small
     \caption{Year of birth statistics for the study cohort}
     \begin{tabular}{c c| c c c c } 
         \toprule
         %\hline
         \textbf{Total Count} & \textbf{Missing} & \textbf{Mean} & \textbf{Std Dev} & \textbf{Min} & \textbf{Max}\\ %[0.5ex] 
         %\hline
         \midrule
         \textbf{72} & 1(1.5\%) & 1941 & 8.24 & 1927 & 1962 \\ 
         %\hline
     \end{tabular}
     \label{tb:YOB_Stats}
\end{table}

\subsection{Minder Study Inclusion and Exclusion Criteria}

Here we detail the comprehensive criteria by which an individual may be included or excluded from the Minder study.

\subsubsection{Inclusion Criteria}

People living with dementia must meet the following criteria to be included in the Minder study:
\vspace{1em}
\begin{itemize}
    \item Have an established dementia of diagnosis or mild cognitive impairment by specialist assessment.
    \item Be male or female over the age of 50 years old.
    \item Have sufficient functional English to allow completion of the assessment instruments.
    \item If lacking in capacity, participants must have a personal consultee representative.
    \item Have a study partner over the age of 18, with sufficient functional English, willing and able to provide informed consent and who has known the person living with dementia for at least 6 months and is able to attend research assessments with them.
\end{itemize}
\vspace{1em}
\subsubsection{Exclusion criteria}

People living with dementia who meet the following criteria are excluded from the Minder study:
\vspace{1em}
\begin{itemize}
    \item Are in receipt of any investigational drug within a 30-day period prior to consenting.
    \item Have an unstable mental state including severe depression, severe psychosis, agitation, and anxiety whose medication was changed over the last 4 weeks.
    \item Have a severe sensory impairment.
    \item Have active suicidal ideation. 
    \item Require regular elective hospital admission for monitoring of their physical health.
    \item Are receiving treatment for a terminal illness.
    \item Have study partners who are unable to communicate verbally or provide written informed consent.
\end{itemize}
